# Supplementary material for: MCgrid: projecting cross section calculations on grids
Source: arXiv:1312.4460 source file (2013-12-16)
Supplement: Supplementary file 1 [file appendix.tex]

\clearpage
\section{Subprocess Identification Scripts}
The subprocess identification config files of \appl list the partonic components of each of the $N_{sub}$ distinct subprocesses present in the calculation. For each subprocess there are a set of $N_{pair}^{(isub)}$ parton-parton pairs that contribute to it. The configuration file denotes these as so:

\begin{lstlisting}[language=bash]
[Flag for removal of CKM matrix elements = 0 or 1]
0 [pair1] [pair2] .. [pairN_0]
1 [pair1] [pair2] .. [pairN_1]
..
[Nsub]  
\end{lstlisting}
Where the pairs are denoted by integer pairs in the \emph{LHA} basis, neglecting the top quark:\\
\begin{table}[h]
\centering
\begin{tabular}{c c c c c c c c c c c }
  $\bar{b}$ & $\bar{c}$ & $\bar{s}$ & $\bar{u}$ & $\bar{d}$ & $g$ & $d$ & $u$ & $s$ & $c$ & $b$ \\
  -5 & -4 & -3 & -2 & -1 & 0 & 1 & 2 & 3 & 4 & 5 \\
\end{tabular}
\end{table}

In \packagename the first parameter in the configuration should always be set to zero, as the \appl functionality of CKM matrix element variations is not available in the package. However the loss of this feature will only impact calculations where the CKM elements enter only in the vertex connecting the two incoming partons. 

As an example configuration, consider a hypothetical process who's only partonic subprocesses consist of $U\bar{U}$ and $gD$ channels where $U$ denotes an up-type quark and $D$ a down-type. The configuration file for \appl would then be:
\begin{lstlisting}[language=bash]
0 
0 2 -2 4 -4 # UUBar
1 0 1 0 3 0 5 # gD
\end{lstlisting}
An important point is that these configuration files refer to the numbering scheme for \emph{proton} distributions. In the case where the user wishes to use a calculation with an initial state antiproton beam, the signs on the antiproton beam flavours should be flipped. For example, for a $p\bar{p}$ beam our previous configuration file would become:
\begin{lstlisting}[language=bash]
0
0 2 2 4 4 # UUBar (ppbar)
1 0 -1 0 -3 0 -5 # gD (ppbar)
\end{lstlisting}
Such that the correct PDF treatment of the antiproton beam is taken into account. 

Provided in the \packagename package are a pair of simple python scripts for the automated generation of \appl \lstinline[language=c++]{lumi_pdf} configuration files from the output of either of the two matrix element generators present in \Sherpa, {\tt COMIX}\cite{Gleisberg:2008fv} and {\tt AMEGIC++}\cite{Krauss:2001iv}. The user may choose to either construct the appropriate configuration file by hand or make use of these scripts.
\label{sec:subproc}
